# Supplementary material for: Generating 6-D Trajectories for Omnidirectional Multirotor Aerial Vehicles in Cluttered Environments
Source: arXiv:2404.10392 source file (2024-07-13)
Supplement: Supplementary file 1 [file appendix.tex]

\appendices
\section{Gradient Calculation in Trajectory Optimization} \label{app:gradient_calculation} 

Gradient of the time-regularized smoothness term $\mathcal{J} := J + k_\rho\Vert\mathbf{T}\Vert_1$ can be calculated as follows:
\begin{align}
\allowdisplaybreaks
    & \frac{\partial \mathcal{J}}{\partial \mathbf{c}_i} = 2 \left(\int_0^{T_i} \bm{\beta}^{(s)}(t)\bm{\beta}^{(s)}(t)^{\top} \text{d}t\right) \mathbf{c}_i, \\
    & \frac{\partial \mathcal{J}}{\partial T_i} = \mathbf{c}_i^{\top}\bm{\beta}^{(s)}(t)\bm{\beta}^{(s)}(t)^{\top}\mathbf{c}_i + k_\rho.
\end{align}

For the penalty terms, each of them is the summary of several sub-penalty terms. 
When the constraint corresponding to a sub-penalty is satisfied, the sub-penalty and its gradient are always 0. 
So we only need to consider the sub-penalties that violate their corresponding constraints,
and we denote them as 
\begin{align}
    & P_{v_{ij}} := \left(\Vert \dot{\mathbf{p}}(\hat{t}_{ij}) \Vert_2^2 - v_{\text{max}}^2\right)^3 \frac{T_i}{\kappa} = \mathcal{G}_{v_{ij}}^3 \frac{T_i}{\kappa}, \\
    & P_{a_{ij}} := \left(\Vert \ddot{\mathbf{p}}(\hat{t}_{ij}) \Vert_2^2 - a_{\text{max}}^2\right)^3 \frac{T_i}{\kappa} = \mathcal{G}_{a_{ij}}^3 \frac{T_i}{\kappa}, \\
    & P_{\omega_{ij}} := \left(\Vert \bm{\omega}(\hat{t}_{ij}) \Vert_2^2 - \omega_{\text{max}}^2\right)^3 \frac{T_i}{\kappa} = \mathcal{G}_{\omega_{ij}}^3 \frac{T_i}{\kappa}, \\
    & P_{c_{ijlk}} := \left(\mathbf{n}_{i, k}^{\top} \left(\mathbf{p}(\hat{t}_{ij}) + \mathbf{R}(\hat{t}_{ij})\tilde{\bm{v}}_l\right) - d_{i, k}\right)^3 \frac{T_i}{\kappa} = \mathcal{G}_{c_{ijlk}}^3 \frac{T_i}{\kappa}. 
\end{align}

Obviously, the penalty terms corresponding to the $i$-th piece are only related to $\mathbf{c}_i$ and $T_i$. 
Then, the expressions are given as follows:% \begin{subequations}
\begin{subequations}
    \allowdisplaybreaks
    \begin{align}
        & \frac{\partial P_{v_{ij}}}{\partial \mathbf{c}_i} = \begin{bmatrix}
            \frac{6T_i}{\kappa} \mathcal{G}_{v_{ij}}^2 \bm{\beta}^{(1)}(\frac{j}{\kappa}T) \dot{\mathbf{p}}^{\top} &
            \mathbf{0}_{2s \times 3}
        \end{bmatrix}, \\
        & \frac{\partial P_{v_{ij}}}{\partial T_i} = \frac{\mathcal{G}_{v_{ij}}^2}{\kappa} \left(\mathcal{G}_{v_{ij}} + \frac{6jT_i}{\kappa}\dot{\mathbf{p}}^{\top}\ddot{\mathbf{p}}\right), \\
        & \frac{\partial P_{a_{ij}}}{\partial \mathbf{c}_i} = \begin{bmatrix}
            \frac{6T_i}{\kappa} \mathcal{G}_{a_{ij}}^2 \bm{\beta}^{(2)}(\frac{j}{\kappa}T) \ddot{\mathbf{p}}^{\top} &
            \mathbf{0}_{2s \times 3}
        \end{bmatrix}, \\
        & \frac{\partial P_{a_{ij}}}{\partial T_i} = \frac{\mathcal{G}_{a_{ij}}^2}{\kappa} \left(\mathcal{G}_{a_{ij}} + \frac{6jT_i}{\kappa}\ddot{\mathbf{p}}^{\top}\dddot{\mathbf{p}}\right), \\
        & \frac{\partial P_{\omega_{ij}}}{\partial \mathbf{c}_i} = \begin{bmatrix}
            \mathbf{0}_{2s \times 3} &
            \frac{6T_i}{\kappa} \mathcal{G}_{\omega_{ij}}^2 \left(\omega_x \frac{\partial \omega_x}{\partial \mathbf{c}_i^\sigma} + \omega_y \frac{\partial \omega_y}{\partial \mathbf{c}_i^\sigma} + \omega_z \frac{\partial \omega_z}{\partial \mathbf{c}_i^\sigma}\right) 
        \end{bmatrix}, \label{equ:Pomg_d_cis} \\
        & \frac{\partial P_{\omega_{ij}}}{\partial T_i} = \frac{\mathcal{G}_{\omega_{ij}}^2}{\kappa} \left(\mathcal{G}_{\omega_{ij}} + \frac{6T_i}{\kappa}\frac{\partial \bm{\omega}}{\partial T_i}\bm{\omega}\right), \label{equ:Pomg_d_Ti} \\
        & \frac{\partial P_{c_{ijlk}}}{\partial \mathbf{c}_i^p} = \frac{3T_i}{\kappa} \mathcal{G}_{c_{ijlk}}^2 \bm{\beta}(\frac{j}{\kappa}T_i)\mathbf{n}_{i, k}^{\top}, \\
        & \left[\frac{\partial P_{c_{ijlk}}}{\partial \mathbf{c}_i^\sigma}\right]_{m, n} = \frac{3T_i}{\kappa} \mathcal{G}_{c_{ijlk}}^2 \mathbf{n}_{i, k}^{\top}\frac{\partial \mathbf{R}}{\partial [\mathbf{c}_i^\sigma]_{m,n}}\tilde{\bm{v}}_l,  \label{equ:Pc_d_cis} \\
        & \begin{aligned}
            & \frac{\partial P_{c_{ijlk}}}{\partial T_i} = \\
            & \frac{\mathcal{G}_{c_{ijlk}}^2}{\kappa} \left[\mathcal{G}_{c_{ijlk}} + 3T_i\left(\frac{j}{\kappa}\mathbf{n}_{i, k}^{\top}{\mathbf{c}_i^p}^{\top}\bm{\beta}^{(1)}(\frac{j}{\kappa}T_i) + \mathbf{n}_{i, k}^{\top}\frac{\partial \mathbf{R}}{\partial T_i}\tilde{\bm{v}}_l\right)\right],  \label{equ:Pc_d_Ti}
        \end{aligned}
    \end{align}
\end{subequations}
where $\mathbf{p}$, $\mathbf{R}$, $\bm{\omega}$, and their derivatives are taken as the values at $\hat{t}_{ij}$;
$[\mathbf{F}]_{m, n}$ is the entry of matrix $\mathbf{F}$ with row index $m$ and column index $n$ and $m \in \{1, \cdots, 2s\}, n \in \{1, \cdots, 6\}$.
